# Supplementary material for: Carbon Explorer: A Holistic Approach for Designing Carbon Aware Datacenters
Source: arXiv:2201.10036 source file (2023-02-22)
Supplement: Supplementary file 1 [file appendix.tex]

\appendix

\begin{figure*}
\centering
\includegraphics[width=1.6\columnwidth]{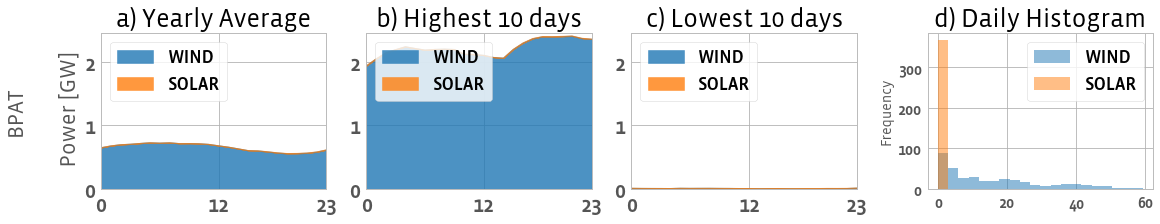}
\includegraphics[width=1.6\columnwidth]{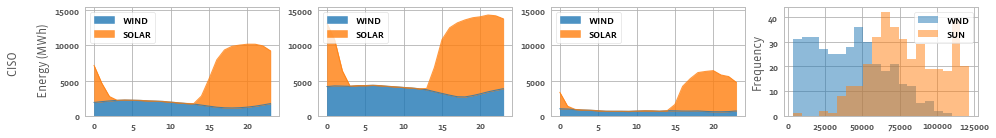}
\includegraphics[width=1.6\columnwidth]{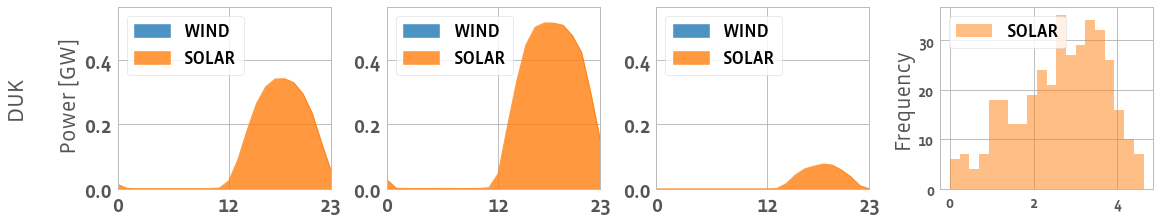}
\includegraphics[width=1.6\columnwidth]{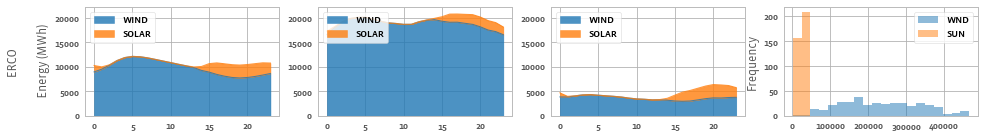}
\includegraphics[width=1.6\columnwidth]{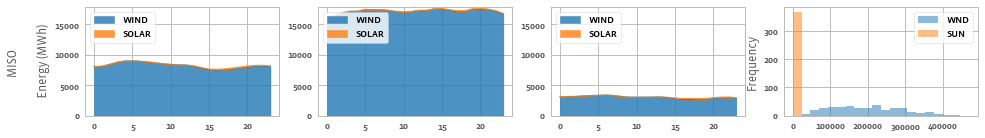}
\includegraphics[width=1.6\columnwidth]{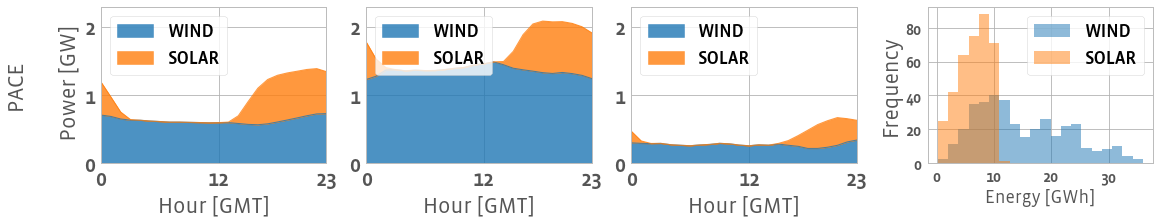}
\includegraphics[width=1.6\columnwidth]{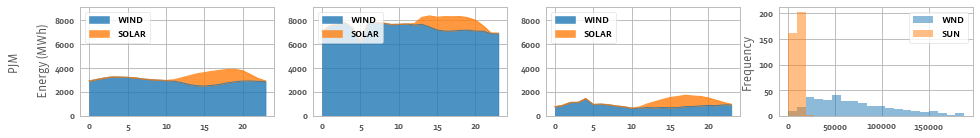}
\includegraphics[width=1.6\columnwidth]{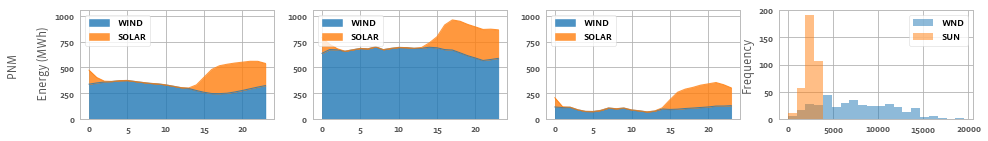}
\includegraphics[width=1.6\columnwidth]{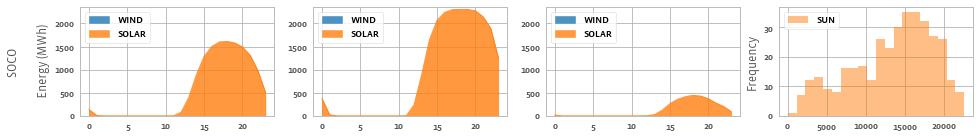}
\includegraphics[width=1.6\columnwidth]{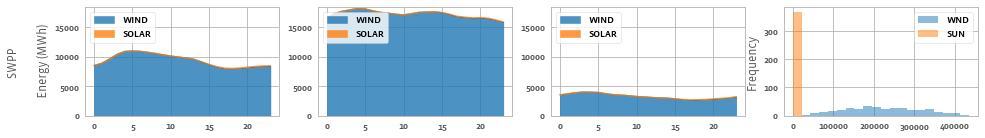}
\includegraphics[width=1.6\columnwidth]{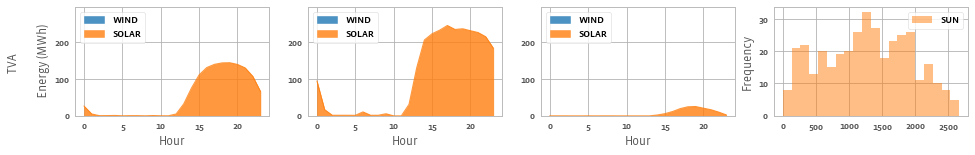}
\caption{Figure shows hourly and seasonal fluctuations of wind and solar generation in all BAs.}
\end{figure*}[ht]

\begin{table}
\centering
\caption{Balancing Authority Acronyms}
\label{ba_names}
\begin{tabular}{c|c}
\textbf{Acronym} & \textbf{Name} \\
\hline
BPAT & Bonneville Power Administration \\
\hline
DUK & Duke Energy Carolinas \\
\hline
MISO & Midcontinent Independent System Operator \\
\hline
PACE & PacificCorp East \\
\hline
PJM & PJM Interconnection LLC \\
\hline
PNM & Public Service Company of New Mexico \\
\hline
SOCO & Southern Company Services \\
\hline
SWPP & Soutwest Power Pool \\
\hline
TVA & Tennessee Valley Authority \\
\end{tabular}
\end{table}
